# Supplementary material for: Scalable 3D Captioning with Pretrained Models
Source: arXiv:2306.07279 source file (2023-06-16)
Supplement: Supplementary file 1 [file datasheet.tex]

Datasheets for Datasets~\citet{gebru2018datasheets} is a standardized documentation process for machine learning datasets. It consists of detailing dataset components including motivation, composition, collection. It has the goal of facilitating communication to dataset users and providing transparency and accountability. 
In this section, we provide a datasheet for this dataset.

\section*{Motivation}

\begin{compactenum}[\hspace{0pt}Q1.]
\setcounter{enumi}{0}

\dsquestionex{For what purpose was the dataset created?}{Was there a specific task in mind? Was there a specific gap that needed to be filled? Please provide a description.}
\label{Q1}

\dsanswer{
    Cap3D captions on Objaverse~\cite{deitke2022objaverse} was collected to facilitate the creation of 3D objects given input text. 
    This was motivated by three observations: (1) publicly available large-scale, high-quality text-image paired data~\cite{schuhmann2022laion,changpinyo2021conceptual,radford2021learning} has transformed text-to-image generation~\cite{ramesh2021zero,gafni2022make,saharia2022photorealistic,rombach2022high,nichol2021glide,ramesh2022hierarchical}; (2) large-scale, high-quality text-3D data (and models) does not publicly exist; (3) large-scale 3D object data is now available~\cite{deitke2022objaverse}.
    By captioning this data and releasing publicly, we hope to facilitate similar progress in text-to-3D generation.
    We also collect human captions, which are used as a baseline for automated captions.
}

\dsanswer{
    We also collect ABO~\cite{collins2022abo} captions. These are collected not with the goal of large-scale text-to-3D generation. Instead, the focus is to measure the ability of automated captioning, which is used in collecting Objaverse captions, to generalize to a focus on object compositional geometry; as well as to measure the ability of prompt engineering to improve captioning performance to describe geometry.
    We also collect human captions, which are used as a baseline for automated captions.
}

\dsquestion{Who created this dataset (e.g., which team, research group) and on behalf of which entity (e.g., company, institution, organization)?}
\label{Q2}

\dsanswer{
    Four University of Michigan researchers created this dataset: Tiange Luo, Chris Rockwell, Honglak Lee, and Justin Johnson. Honglak is also affiliated with LG AI Research.
}

\dsquestionex{Who funded the creation of the dataset?}{If there is an associated grant, please provide the name of the grantor and the grant name and number.}
\label{Q3}

\dsanswer{
    This work is supported by two grants from LG AI Research and Grant #1453651 from NSF.
    %We collected \dsetname{} without any monetary costs, since no part of our dataset %requires annotations from crowd workers or contractors.
    %This research work was partially supported by the Toyota Research Institute (TRI).
    %However, note that this article solely reflects the opinions and conclusions of its %authors and not TRI or any other Toyota entity.
}

\dsquestion{Any other comments?}
\label{Q4}

\dsanswer{No.}

\end{compactenum}

%%%%%%%%%%%%%%%%%%%%%%%%%%%%%%%%%%%%%%%%%%%%%%%%%%%%%%%%%%%%%%%%%%%%%%%%%%%%%%

\section*{Composition}

\begin{compactenum}[\hspace{0pt}Q1.]
\setcounter{enumi}{4}
    
\dsquestionex{What do the instances that comprise the dataset represent (e.g., documents, photos, people, countries)?}{ Are there multiple types of instances (e.g., movies, users, and ratings; people and interactions between them; nodes and edges)? Please provide a description.}
\label{Q5}

\dsanswer{Objaverse. Each captioning instance represents an object paired with a caption describing the structure, appearance and class of the object. There is one automated caption per object. Human captions may contain multiple captions per object.
}

\dsanswer{ABO. Each captioning instance represents an object paired with a caption describing the compositional geometry and class of the object. Human captions may contain multiple captions per object.
}

\dsquestion{How many instances are there in total (of each type, if appropriate)?}
\label{Q6}

\dsanswer{Objaverse. There are 660k instances. Human captions have 41k captions spanning 39k objects.
}

\dsanswer{ABO. There are 6.4k automated captions, and 17k human captions corresponding to 6.4k objects.
}

\dsquestionex{Does the dataset contain all possible instances or is it a sample (not necessarily random) of instances from a larger set?}{ If the dataset is a sample, then what is the larger set? Is the sample representative of the larger set (e.g., geographic coverage)? If so, please describe how this representativeness was validated/verified. If it is not representative of the larger set, please describe why not (e.g., to cover a more diverse range of instances, because instances were withheld or unavailable).}
\label{Q7}

\dsanswer{Objaverse. This dataset consists of captions on the entirety of a subset of the Objaverse dataset. The total size is 660k objects of the original 798k. Our subset is filtered to include only the CC-BY 4.0, CC-BY-NC 4.0 and CC0 1.0 licenses (CC-BY-SA 4.0 and CC-BY-NC-SA 4.0 are excluded). We further exclude objects without sufficient camera information for rendering. We finally remove NSFW images and captions, along with visible faces. The subset is not totally representative of the full set, as the full set contains more NSFW content and faces. The filters are made to instead make the dataset more widely accessible.
}

\dsanswer{ABO. We use the same subset as \cite{luo2023neural}, which removes objects with little interesting geometry. We do not filter further, as the dataset does not contain NSFW content or faces, and falls under CC-BY-NC 4.0, so we do not filter based on licensing.
}

\dsquestionex{What data does each instance consist of? “Raw” data (e.g., unprocessed text or images) or features?}{In either case, please provide a description.}
\label{Q8}

\dsanswer{Objaverse. Each instance consists of seven metadata fields:
    \begin{compactitem}
        \item \texttt{"uid"}: Objaverse-assigned unique ID of the object. 
        \item \texttt{"images"}: List of rendered images.
        \item \texttt{"cameras"}: List of camera parameters for each rendered image used to collect captions.
        \item \texttt{"captions"}: List where each element corresponds to an image in \textit{"images"}. 
        \item \texttt{"point cloud"}: List of rendered images.
        \item \texttt{"latent code"}: Shap·E latent code, used to finetune Shap·E.
    \end{compactitem}
}

\dsanswer{ABO. Each instance consists of two metadata fields:
    \begin{compactitem}
        \item \texttt{id}: ABO-assigned unique ID of the object. We do not hold any object information (e.g. 3D asset or rendered image) from ABO; this can be used in conjunction with the ABO API.
        \item \texttt{"captions"}: List where each element contains a caption.
    \end{compactitem}
}

\dsquestionex{Is there a label or target associated with each instance?}{If so, please provide a description.}
\label{Q9}

\dsanswer{Objaverse. If performing text-to-3D, the target for each \textit{"uid"} is the corresponding 3D \textit{"point cloud"}.% This object is saved as a \textit{".glb"} file and can be (1) rendered to measure 3D texture/color quality, or (2) sampled from to measure reconstruction accuracy. However, 
The collected caption data can be used for other purposes, such as: text-to-image generation (\textit{input: captions, target: rendered images}), 3D captioning (\textit{input: set of rendered images or point cloud, target: caption}), image captioning (\textit{input: rendered image, target: captions}).
}

\dsanswer{ABO. We do not perform text-to-3D on ABO, but assets exist corresponding to captions, which could be used as target.}
}

\dsquestionex{Is any information missing from individual instances?}{If so, please provide a description, explaining why this information is missing (e.g., because it was unavailable). This does not include intentionally removed information, but might include, e.g., redacted text.}
\label{Q10}

\dsanswer{Objaverse and ABO. No.}

\dsquestionex{Are relationships between individual instances made explicit (e.g., users’ movie ratings, social network links)?}{If so, please describe how these relationships are made explicit.}
\label{Q11}

\dsanswer{Objaverse. A number of relationships exist between instances in our data. For example: multiple objects may have the same artist, objects can be of the same category of object (e.g. furniture), or even the same object type (e.g. chair). This information is captured to some extent in the Objaverse metadata, to which we provide a lookup. However, Objaverse metadata is incomplete for many objects, meaning relationships between instances are not always explicit. 
}

\dsanswer{ABO. Inferring relationships between instances may not be easy, beyond looking into captions or basic metadata. Metadata tends to be very limited.
}

\dsquestionex{Are there recommended data splits (e.g., training, development/validation, testing)?}{If so, please provide a description of these splits, explaining the rationale behind them.}
\label{Q12}

\dsanswer{Objaverse. Yes. We provide splits for text-to-3D, with a special 300-object split for optimization-based methods.}

\dsanswer{ABO. Yes, the splits of ~\cite{luo2023neural}.
}

\dsquestionex{Are there any errors, sources of noise, or redundancies in the dataset?}{If so, please provide a description.}
\label{Q13}

\dsanswer{Objaverse and ABO. The caption dataset is generated using a learned image captioning model upon a variety of rendered images, followed by a learned text summarization model. There are therefore several sources of possible error, including: (1) objects may be out-of-domain for the captioning model, leading to incorrect captions; (2) rendered images may vary in scale and orientation to objects, leading to uninformative rendered images; (3) captions may be out-of-domain for the text summarization model, leading to summarizations including incorrect details or excluding correct details. However, in practice we show these errors are less frequent and less meaningful than human annotators, meaning the proposed captioning approach is still highly effective. During manual exploration of tens of thousands of objects, we noticed some duplicate objects in Objaverse. However, these were infrequent. In contrast, ABO contains a high number of very similar objects.
}

\dsquestionex{Is the dataset self-contained, or does it link to or otherwise rely on external resources (e.g., websites, tweets, other datasets)?}{If it links to or relies on external resources,
\begin{compactenum}[\hspace{1pt}(a)]
    \item Are there guarantees that they will exist, and remain constant, over time?
    \item Are there official archival versions of the complete dataset (i.e., including the external resources as they existed at the time the dataset was created)?
    \item Are there any restrictions (e.g., licenses, fees) associated with any of the external resources that might apply to a future user? Please provide descriptions of all external resources and any restrictions associated with them, as well as links or other access points, as appropriate.
\end{compactenum}}
\label{Q14}

\dsanswer{Objaverse. The dataset is self-contained, while additionally providing keys mapping to assets contained in the external Objaverse dataset. We make this choice to (1) facilitate replicability, (2) promote integration with external Objaverse information.
    \begin{compactenum}[\hspace{1pt}(a)]
        \item Our data, as well as Objaverse, is released under the ODC-By 1.0 license meaning it should be stable unless users request their assets be removed.
        \item Yes, please see (1) our captions at \url{https://huggingface.co/datasets/tiange/Cap3D}, which provides directions to use (2) 3D assets at \url{https://objaverse.allenai.org/docs/download}. Upon updates, our assets will be archived unless they are removed at author request or for future ethical reasons. 
        \item External 3D assets for our dataset are available at \url{https://objaverse.allenai.org/docs/download}. As of our release, the external assets are licensed under CC-BY 4.0, CC-BY-NC 4.0 and CC0 1.0, and do not have a fee associated. It is unlikely they will have a fee in the future considering the associated license.
    \end{compactenum}
}

\dsanswer{ABO. Our ABO captions are associated with an ID that can be used to obtain objects and real renders of ABO objects.
\begin{compactenum}[\hspace{1pt}(a)]
    \item Our data, as well as ABO, is released under the CC BY-NC 4.0 license meaning it should be stable unless users request their assets be removed.
    \item Yes, please see (1) our captions at \url{https://huggingface.co/datasets/tiange/Cap3D}, which provides directions to use (2) 3D assets at \url{https://amazon-berkeley-objects.s3.amazonaws.com/index.html}. Upon updates, our assets will be archived unless they are removed at author request or for future ethical reasons. 
    \item There is no current fee, and it is unlikely there will be a fee in the future with external resources (\url{https://amazon-berkeley-objects.s3.amazonaws.com/index.html}) due to the CC BY-NC 4.0 license associated.
\end{compactenum}
}

\dsquestionex{Does the dataset contain data that might be considered confidential (e.g., data that is protected by legal privilege or by doctor-patient confidentiality, data that includes the content of individuals non-public communications)?}{If so, please provide a description.}
\label{Q15}

\dsanswer{Objaverse and ABO. The collected captions are generated using a model~\cite{li2023blip} trained upon datasets which are publicly available, and are thus unlikely to include confidential information: COCO~\cite{lin2014microsoft}, Visual Genome~\cite{krishna2017visual}, CC3M~\cite{sharma2018conceptual}, CC12M~\cite{changpinyo2021conceptual}, SBU~\cite{ordonez2011im2text}, LAION400M~\cite{schuhmann2021laion}. For instance, a recent study of LAION400M found NSFW information, but does not report finding confidential information~\cite{birhane2021multimodal}. 
An analysis of NSFW-related questions will be discussed in \ref{Q16}. 
As the captioning model is trained on datasets without confidential information, it is reasonable to expect the model would not generate confidential information. 
On Objaverse, we further run a face detector to minimize personally identifiable information.
On ABO, we manually verify no faces occur in the dataset.
}


\dsquestionex{Does the dataset contain data that, if viewed directly, might be offensive, insulting, threatening, or might otherwise cause anxiety?}{If so, please describe why.}
\label{Q16}

\dsanswer{Objaverse. The scale of Objaverse makes it difficult to manually verify all data. However, we run a standard NSFW detector~\cite{desai2021redcaps,deng2020retinaface} on images and standard blocklist~\cite{dirty23} on captions. 
We manually estimate precision and recall of these methods in \S ~\ref{sec:method_filtering}, and estimate less than 1k NSFW content remains in the full dataset, by a conservative standard.
}

\dsanswer{ABO. ABO consists of furniture and is of small scale. Manual verification finds no offensive objects. We run a standard blocklist on captions, and verifies 3DCap captions contain NSFW content.
}

\dsquestionex{Does the dataset relate to people?}{If not, you may skip remaining questions in this section.}
\label{Q17}

\dsanswer{Objaverse. A small proportion (<1\%) of the dataset contains real people. However, we attempt to minimize possible people by applying a face detector and removing detected faces. Details and analysis are available in \S ~\ref{sec:method_filtering}. To summarize, after filtering, about 1k people may remain, although the vast majority of instances are publicly available sports cards. Due to the limited nature of this data in the entire dataset, we provide further analysis to the best of our abilities.
    %\crnote{probably want to remove people so we can skip these}
    %\answerTODO{}
    %The dataset pertains to people in that people wrote the captions and posted images to Reddit that we curate in \dsetname{}.
    %We made specific design choices while curating \dsetname{} to avoid large quantities of images containing people:
    %\begin{compactenum}
    %    \item We collect data from manually curated subreddits in which most contain primarily pertains to animals, objects, places, or activities.
    %    We exclude all subreddits whose primary purpose is to share and describe images of people (such as celebrity photos or user selfies).
    %    \item We use an off-the-shelf face detector to find and remove images with potential presence of human faces.
    %    We manually checked 50K random images in \dsetname{} (\qref{Q16}) and found 79 images with identifiable human faces -- the entire dataset may have $\approx$19K (0.15\%) images with identifiable people.
    %    Refer \textcolor{Red}{Section 2.2} in the main paper.
    %\end{compactenum}
}

\dsanswer{ABO. No, it is of only furniture.
}

\dsquestionex{Does the dataset identify any subpopulations (e.g., by age, gender)?}{If so, please describe how these subpopulations are identified and provide a description of their respective distributions within the dataset.}
\label{Q18}

\dsanswer{Objaverse. It does not explicitly identify subpopulations.}

\dsanswer{ABO. N/A.
}

%\dsanswer{
%    \answerTODO{}
%
%    \dsetname{} does not explicitly identify any subpopulations.
%    Since some images contain people and captions are free-form natural language written by Reddit users, it is possible that some captions may identify people appearing in individual images as part of a subpopulation.
%}

%\dsanswer{ABO. N/A.
%}

\dsquestionex{Is it possible to identify one or more natural persons, either directly or indirectly (i.e., in combination with other data) from the dataset?}{If so, please describe how.}
\label{Q19}

\dsanswer{Objaverse. Yes - the vast majority of real people appearing in the dataset are publicly available sports cards, which consist of a name as well as a photograph of the athlete.}

\dsanswer{ABO. N/A.
}

%\dsanswer{
%    \answerTODO{} Very unlikely. The 
%
%    Yes, all instances in \dsetname{} include Reddit usernames of their post authors.
%    This could be used to look up the Reddit user profile, and some Reddit users may have identifying information in their profiles.
%    Some images may contain human faces (\qref{Q17}) which could be identified by appearance.
%    However, note that all this information is already public on Reddit, and searching it in \dsetname{} is no easier than searching directly on Reddit.
%}

%\dsanswer{ABO.\answerTODO{}
%}

\dsquestionex{Does the dataset contain data that might be considered sensitive in any way (e.g., data that reveals racial or ethnic origins, sexual orientations, religious beliefs, political opinions or union memberships, or locations; financial or health data; biometric or genetic data; forms of government identification, such as social security numbers; criminal history)?}{If so, please provide a description.}
\label{Q20}

%\dsanswer{
%    Highly unlikely, the data from our manually selected subreddits does not contain sensitive information of the above forms.
%    In case some instances have such information, then note that all this information is already publicly available on Reddit.
%}

%\dsanswer{ABO.\answerTODO{}
%}

\dsanswer{Objaverse. A manual search of over 10k objects did not find any of this information in images. It is highly unlikely these would occur on 3D assets, while captions are trained on publicly available data, and are filtered via GPT4 and a blocklist (see \S ~\ref{sec:method_filtering}), making this very unlikely.}

\dsanswer{ABO. N/A.
}

\dsquestion{Any other comments?}
\label{Q21}

\dsanswer{Objaverse and ABO. No.
}

\end{compactenum}

%%%%%%%%%%%%%%%%%%%%%%%%%%%%%%%%%%%%%%%%%%%%%%%%%%%%%%%%%%%%%%%%%%%%%%%%%%%%%%

\section*{Collection Process}

\begin{compactenum}[\hspace{0pt}Q1.]
\setcounter{enumi}{21}

\dsquestionex{How was the data associated with each instance acquired?}{Was the data directly observable (e.g., raw text, movie ratings), reported by subjects (e.g., survey responses), or indirectly inferred/derived from other data (e.g., part-of-speech tags, model-based guesses for age or language)? If data was reported by subjects or indirectly inferred/derived from other data, was the data validated/verified? If so, please describe how.}
\label{Q22}

\dsanswer{Objaverse and ABO. Automated collection is detailed in \S ~\ref{sec:method_captioning}.
Human collection is detailed in \S ~\ref{sec:dataset_obja}.
To summarize, automated captioning applies three pretrained models to rendered images, while we use {\href{https://thehive.ai/}{Hive}} for human captions. Both are followed by ethical filtering (\S ~\ref{sec:method_filtering}). 
}

\dsquestionex{What mechanisms or procedures were used to collect the data (e.g., hardware apparatus or sensor, manual human curation, software program, software API)?}{How were these mechanisms or procedures validated?}
\label{Q23}

\dsanswer{Objaverse and ABO. 
%All automated data was collected using University of Michigan's computing resources (e.g. BLIP2 runs on A40 GPU; rendering was performed across a variety of modern GPUs). Code is implemented in Python. Data collection was manually verified throughout collection, and is ultimately validated through extensive experiments in the paper. Human annotation used \url{thehive.ai}, a crowd-sourced worker site similar to AMT. 
Automated captions were collected using A40 GPUs for BLIP2 and CLIP; rendering was performed across a variety of modern GPUs, and we use OpenAI's API to access GPT4.
Code is implemented in Python. 
Human annotation used {\href{https://thehive.ai/}{Hive}}, a crowd-sourced worker site similar to AMT. 
Data collection was manually verified throughout collection, and is validated through extensive experiments in the paper. 
}

\dsquestion{If the dataset is a sample from a larger set, what was the sampling strategy?}
\label{Q24}

\dsanswer{Objaverse and ABO. Beyond filtering in \ref{Q7}, we do not subsample.
}

\dsquestion{Who was involved in data collection process (e.g., students, crowd-workers, contractors) and how were they compensated (e.g., how much were crowd-workers paid)?}
\label{Q25}

\dsanswer{ABO and Objaverse. Our primary captioning is automated using a pretrained image captioning model. 
Human captions are annotated by crowd-workers. They were paid USD \$50 per 1000 object captions.
}

\dsquestionex{Over what timeframe was the data collected? Does this timeframe match the creation timeframe of the data associated with the instances (e.g., recent crawl of old news articles)?}{If not, please provide a description of the timeframe.}
\label{Q26}

\dsanswer{Objaverse. Automated captioning was collected between March - June 2023. Human captioning was collected collected between February - May 2023. The original Objaverse dataset was released in December 2022, meaning captions were obtained shortly after release.
}

\dsanswer{ABO. Human captioning was collected between June 2022 - May 2023. The original ABO dataset was released in October 2021, meaning captions were obtained shortly after release.
}

\dsquestionex{Were any ethical review processes conducted (e.g., by an institutional review board)?}{If so, please provide a description of these review processes, including the outcomes, as well as a link or other access point to any supporting documentation.}
\label{Q27}

\dsanswer{Objaverse and ABO. We did not conduct a formal review process. However, we performed filtering and analysis (~\S \ref{sec:method_filtering}) to minimize potential ethical concerns.
}

\dsquestionex{Does the dataset relate to people?}{If not, you may skip remaining questions in this section.}
\label{Q28}

%\dsanswer{
%    Some images of \dsetname{} may contain images of people (see \qref{Q17}).
%}

%\dsanswer{ABO.\answerTODO{}
%}
\dsanswer{Objaverse. Yes - the objects in Objaverse were created by over 100k artists, all released under public licenses.}

\dsanswer{ABO. No - the objects in ABO are credit of Amazon.com.
}

\dsquestion{Did you collect the data from the individuals in question directly, or obtain it via third parties or other sources (e.g., websites)?}
\label{Q29}

%\dsanswer{
%    We collected data submitted by Reddit users indirectly through the Reddit API.
%    However, users agree with Reddit's User Agreement regarding redistribution of their data by Reddit.
%}

\dsanswer{Objaverse. We obtain objects from third party Objaverse, which releases the dataset as a whole under ODC-By 1.0 license. We consider only assets individuals release with the CC BY, CC BY-SA, and CC0 license.
}

\dsanswer{ABO. Data is not the property of individuals, and is released publicly under CC BY-NC 4.0 license.
}

\dsquestionex{Were the individuals in question notified about the data collection?}{If so, please describe (or show with screenshots or other information) how notice was provided, and provide a link or other access point to, or otherwise reproduce, the exact language of the notification itself.}
\label{Q30}

%\dsanswer{
%    No. Reddit users are anonymous by default, and are not required to share their personal contact information (email, phone numbers, etc.).
%    Hence, the only way to notify the authors of \dsetname{} image posts is by sending them private messages on Reddit.
%    This is practically difficult to do manually, and will be classified as spam and blocked by Reddit if attempted to programmatically send a templated message to millions of users.
%}

\dsanswer{Objaverse. While contacting each of 100k authors directly is challenging, Objaverse consists only of objects which users release with the explicit purpose of redistribution (under creative commons distributable licenses).
}

\dsanswer{ABO. N/A.
}

\dsquestionex{Did the individuals in question consent to the collection and use of their data?}{If so, please describe (or show with screenshots or other information) how consent was requested and provided, and provide a link or other access point to, or otherwise reproduce, the exact language to which the individuals consented.}
\label{Q31}

%\dsanswer{
%    Users did not explicitly consent to the use of their data in our dataset.
%    However, by uploading their data on Reddit, they consent that it would appear on the Reddit plaform and will be accessible via the official Reddit API (which we use to collect \dsetname{}).
%}

\dsanswer{Objaverse. Yes, via creative commons distributable license.
}

\dsanswer{ABO. N/A.
}

\dsquestionex{If consent was obtained, were the consenting individuals provided with a mechanism to revoke their consent in the future or for certain uses?}{If so, please provide a description, as well as a link or other access point to the mechanism (if appropriate).}
\label{Q32}

%\dsanswer{
%    Users have full control over the presence of their data in our dataset.
%    If users wish to revoke their consent, they can delete the underlying Reddit post -- it will be automatically removed dfrom \dsetname{} since we distributed images as URLs.
%    Moreover, we provide an opt-out request form on our dataset website for anybody to request removal of an individual instance if it is potentially harmful (e.g. NSFW, violates privacy, harmful stereotypes, etc.).
}
\dsanswer{Objaverse. Both Objaverse and our collected captions are released via Hugging Face: \url{https://huggingface.co/datasets/allenai/objaverse/discussions},  \url{https://huggingface.co/datasets/tiange/Cap3D/discussions}, in which authors can contact authors in the "community" section. Users are also encouraged to reach out to Chris and Tiange through email, which is advertised on the dataset Hugging Face.
}
\dsanswer{ABO. N/A.
}

\dsquestionex{Has an analysis of the potential impact of the dataset and its use on data subjects (e.g., a data protection impact analysis) been conducted?}{If so, please provide a description of this analysis, including the outcomes, as well as a link or other access point to any supporting documentation.}
\label{Q33}

%\dsanswer{No.}

%\dsanswer{ABO.\answerTODO{}
%}
\dsanswer{Objaverse and ABO. N/A.
}

\dsquestion{Any other comments?}
\label{Q34}

\dsanswer{Objaverse and ABO. No.}

\end{compactenum}

%%%%%%%%%%%%%%%%%%%%%%%%%%%%%%%%%%%%%%%%%%%%%%%%%%%%%%%%%%%%%%%%%%%%%%%%%%%%%%

\section*{Preprocessing, Cleaning, and/or Labeling}

\begin{compactenum}[\hspace{0pt}Q1.]
\setcounter{enumi}{34}

\dsquestionex{Was any preprocessing/cleaning/labeling of the data done (e.g., discretization or bucketing, tokenization, part-of-speech tagging, SIFT feature extraction, removal of instances, processing of missing values)?}{If so, please provide a description. If not, you may skip the remainder of the questions in this section.}
\label{Q35}

\dsanswer{Objaverse and ABO. Automated captions are not processed beyond the steps in the automated pipeline described in \S \ref{sec:method_captioning} and \S \ref{sec:method_filtering}. Human captions are filtered to maximize quality. In addition to removing captions from banned workers, we remove captions with 1 or less word, remove duplicate captions of the same object, and remove captions appearing more than 30 times across the dataset for likely scam.
    %We filtered all image posts with $< 2$ net upvotes, and those marked NSFW on Reddit.
    %We remove character accents, emojis, non-latin characters, sub-strings enclosed in brackets (\inlinecap{(.*)}, \inlinecap{[.*]}), and replace social media handles (words starting with `@') with a special \inlinecap{[USR]} token.
   % Refer \textcolor{Red}{Section 2.1} in the main paper for more details.
   % We also remove additional instances with focus on ethical considerations, see 
    %\qref{Q16}, \qref{Q17} for more details.
}

\dsquestionex{Was the ``raw'' data saved in addition to the preprocessed/cleaned/labeled data (e.g., to support unanticipated future uses)?}{If so, please provide a link or other access point to the “raw” data.}
\label{Q36}

\dsanswer{Objaverse and ABO. We do not save filtered human captions, which consist of a small portion of data and generally are not useful captions.
    %We provide the unprocessed captions obtained as-is from Reddit as part of our annotations (see \texttt{``raw\_caption''} in \qref{Q8}).
    %However, we entirely discard all instances that were filtered with ethical considerations -- based on presence of faces, NSFW content, or harmful language.
}

\dsquestionex{Is the software used to preprocess/clean/label the instances available?}{If so, please provide a link or other access point.}
\label{Q37}

\dsanswer{Objaverse and ABO. Yes, this will be released publicly through \url{https://github.com/crockwell/Cap3D}.
    %Yes, the data collection code is open-sourced and accessible from the dataset website.
}

\dsquestion{Any other comments?}
\label{Q38}

\dsanswer{No.}

\end{compactenum}

%%%%%%%%%%%%%%%%%%%%%%%%%%%%%%%%%%%%%%%%%%%%%%%%%%%%%%%%%%%%%%%%%%%%%%%%%%%%%%

\section*{Uses}

\begin{compactenum}[\hspace{0pt}Q1.]
\setcounter{enumi}{38}

\dsquestionex{Has the dataset been used for any tasks already?}{If so, please provide a description.}
\label{Q39}

\dsanswer{Objaverse. Yes, the dataset has been used for inference and fine-tuning of existing text to 3D systems and their sub-components. They have trained using paired text, image, and 3D data.
    %We have used our dataset to train deep neural networks that perform image captioning, and that learn transferable visual representations for a variety of downstream visual recognition tasks (image classification, object detection, instance segmentation).
}

\dsanswer{ABO. Not beyond caption validation.
}

\dsquestionex{Is there a repository that links to any or all papers or systems that use the dataset?}{If so, please provide a link or other access point.}
\label{Q40}

\dsanswer{Objaverse and ABO. No current cite exists, though we encourage dataset users to cite us. Google Scholar maintains a citation network. 
}

\dsquestion{What (other) tasks could the dataset be used for?}
\label{Q41}

\dsanswer{Objaverse and ABO. Text-to-image generation, 3D captioning, image captioning. Like Objaverse, ABO can be used for text-to-3D generation.
}

\dsquestionex{Is there anything about the composition of the dataset or the way it was collected and preprocessed/cleaned/labeled that might impact future uses?}{For example, is there anything that a future user might need to know to avoid uses that could result in unfair treatment of individuals or groups (e.g., stereotyping, quality of service issues) or other undesirable harms (e.g., financial harms, legal risks) If so, please provide a description. Is there anything a future user could do to mitigate these undesirable harms?}
\label{Q42}

\dsanswer{Objaverse. It is difficult to image all ways the dataset could be used and give users blanket advice. 
Users should be aware Objaverse consists of artist-created assets that can depict characters and objects which could be linked to NSFW or biased content, even if the apparent asset itself is not NSFW or biased. 
Given the scale (>700k objects) it is difficult to consider each object on a case-by-case basis, and even if so, different interpretations may lead to people feeling emotionally harmed even if it is not originally clear to the creators or when filtering data. 
Artist-created assets also reflect the interests of artists, which isn't to create objects reflective of those used by all demographics, countries, etc. 
This is therefore a biased collection of objects. 
In addition, the automated captioning model is trained on massive amounts of internet data, which can include NSFW and biased content~\cite{birhane2021multimodal}; while humans are also biased and sometimes produce NSFW captions.
As a result, the text-3D pairs could contain NSFW or biased content. Nevertheless, we combat this by filtering bad examples, and analyze remaining objects. 
Our manual random sample of 10k objects finds 12 instances of NSFW content after filtering, by a conservative standard. 
Beyond manually filtering data further, future users could further filter model outputs trained upon this data. 
To combat bias, Objaverse objects could be filtered by metadata or captions into known subsets, so outputs are more consistent with user expectations.
%    This is very difficult to anticipate.
%    Future users of our dataset should be aware of Reddit's user demographics (as described in \textcolor{Red}{Section 2.2} of the main paper) which might subtly influence the types of images, languages, and ideas that are present in the dataset.
%    Moreover, users should be aware that our dataset intentionally excludes data from subreddits whose primary purpose is to share images that depict or describe people.
}

\dsanswer{ABO. ABO consists of products Amazon sells. Since Amazon does not sell equally by demographic, country or any number of other factors, these objects are a biased selection. 
ABO text annotations that are labeled by humans, or automatically generated, can be biased or produce bad captions.
We filter NSFW using a blocklist. 
For users to minimize impact of ABO biases, we recommend filtering further by caption or metadata into known subsets, so outputs are more consistent with user expectations.
}

\dsquestionex{Are there any tasks for which the dataset should not be used?}{If so, please provide a description.}
\label{Q43}

\dsanswer{Objaverse and ABO. It is difficult to exhaustively list negative applications of internet data. One task it should clearly not be used for is for unethical purposes, such as those relating to personal identity, or for making decisions about people (e.g. mortgage application).
    %Broadly speaking, our dataset should only be used for non-commercial academic research.
    %Our dataset should not be used for any tasks that involve identifying features related to people (facial recognition, gender, age, ethnicity identification, etc.) or make decisions that impact people (mortgages, job applications, criminal sentences; or moderation decisions about user-uploaded data that could result in bans from a website).
    %Any commercial and for-profit uses of our dataset are restricted -- it should not be used to train models that will be deployed in production systems as part of a product offered by businesses or government agencies.
}

\dsquestion{Any other comments?}
\label{Q44}

\dsanswer{Objaverse and ABO. No.}

\end{compactenum}

%%%%%%%%%%%%%%%%%%%%%%%%%%%%%%%%%%%%%%%%%%%%%%%%%%%%%%%%%%%%%%%%%%%%%%%%%%%%%%

\section*{Distribution}

\begin{compactenum}[\hspace{0pt}Q1.]
\setcounter{enumi}{44}

\dsquestionex{Will the dataset be distributed to third parties outside of the entity (e.g., company, institution, organization) on behalf of which the dataset was created?}{If so, please provide a description.}
\label{Q45}

\dsanswer{Objaverse and ABO. Yes, the dataset will be publicly available.
}

\dsquestionex{How will the dataset will be distributed (e.g., tarball on website, API, GitHub)}{Does the dataset have a digital object identifier (DOI)?}
\label{Q46}

\dsanswer{Objaverse and ABO. The dataset will be distributed via Hugging Face (\url{https://huggingface.co/datasets/tiange/Cap3D}). Helpful scripts will be available soon via GitHub (\url{https://github.com/crockwell/Cap3D}).
}

\dsquestion{When will the dataset be distributed?}
\label{Q47}

\dsanswer{Objaverse and ABO. The dataset is publicly available as of the NeurIPS Dataset Track supplemental deadline. Github will be available before the camera ready deadline.
}

\dsquestionex{Will the dataset be distributed under a copyright or other intellectual property (IP) license, and/or under applicable terms of use (ToU)?}{If so, please describe this license and/or ToU, and provide a link or other access point to, or otherwise reproduce, any relevant licensing terms or ToU, as well as any fees associated with these restrictions.}
\label{Q48}

\dsanswer{Objaverse. It is released under the ODC-By 1.0 license.
    %Uses of our dataset are subject to Reddit API terms (\url{https://www.reddit.com/wiki/api-terms}).
    %Additionally users must comply with Reddit User Agreeement, Content Policy, and Privacy Policy -- all accessible at \url{https://www.redditinc.com/policies}.
    %The data collection code is released with an MIT license.
}

\dsanswer{ABO. It is released under the CC BY-NC 4.0 license.
}

\dsquestionex{Have any third parties imposed IP-based or other restrictions on the data associated with the instances?}{If so, please describe these restrictions, and provide a link or other access point to, or otherwise reproduce, any relevant licensing terms, as well as any fees associated with these restrictions.}
\label{Q49}

\dsanswer{Objaverse. Objaverse as a whole is released under the ODC-By 1.0 license. We consider only objects with the CC-BY 4.0, CC-BY-NC 4.0 and CC0 1.0 licenses; excluding those with CC-BY-SA 4.0, CC-BY-NC-SA 4.0 licenses. \url{https://opendatacommons.org/licenses} contains simple explanations of licenses.
    %The images corresponding to our instances are legally owned by Reddit users.
    %Our dataset users can download them from the URLs we provide in annotation files, but resdistributing images for commercial use is prohibited.
}

\dsanswer{ABO. ABO is shared via CC-BY-NC 4.0 license from Amazon of their products. 
}

\dsquestionex{Do any export controls or other regulatory restrictions apply to the dataset or to individual instances?}{If so, please describe these restrictions, and provide a link or other access point to, or otherwise reproduce, any supporting documentation.}
\label{Q50}

\dsanswer{Objaverse and ABO. N/A.}

\dsquestion{Any other comments?}
\label{Q51}

\dsanswer{Objaverse and ABO. No.}
% \dsanswer{Objaverse. In addition to ethical filters on data, we will use the NSFW filter of Huggingface Diffusers in the public release of our code, to further reduce NSFW content generated by models trained on our data.}

\end{compactenum}

%%%%%%%%%%%%%%%%%%%%%%%%%%%%%%%%%%%%%%%%%%%%%%%%%%%%%%%%%%%%%%%%%%%%%%%%%%%%%%

\section*{Maintenance}

\begin{compactenum}[\hspace{0pt}Q1.]
\setcounter{enumi}{51}

\dsquestion{Who will be supporting/hosting/maintaining the dataset?}
\label{Q52}

\dsanswer{Objaverse and ABO. The dataset is hosted and will be maintained by Tiange and Chris at \url{https://huggingface.co/datasets/tiange/Cap3D}. This site will also contain information about the dataset, including links to paper and code.
}

\dsquestion{How can the owner/curator/manager of the dataset be contacted (e.g., email address)?}
\label{Q53}

\dsanswer{Objaverse and ABO. The preferred point of contact is the "community" section of the Hugging Face.}

\dsquestionex{Is there an erratum?}{If so, please provide a link or other access point.}
\label{Q54}

\dsanswer{Objaverse and ABO. There is no erratum for our initial release. It will be included in any future versions.
}

\dsquestionex{Will the dataset be updated (e.g., to correct labeling errors, add new instances, delete instances)?}{If so, please describe how often, by whom, and how updates will be communicated to users (e.g., mailing list, GitHub)?}
\label{Q55}

\dsanswer{Objaverse and ABO. We will update if new ethical risks are found. 
Artists will also be able to request to remove captioned objects using the Hugging Face "community" section; which will result in updates. 
%A form will also be available for Objaverse artists or people potentially depicted by Objaverse to request to remove captioned objects; which will result in updates. 
This will be done by Tiange and / or Chris, and updates will be announced on the dataset Hugging Face page.
} %  We will also update if unforeseen and significant ethical issues arise in the current data.

\dsquestionex{If the dataset relates to people, are there applicable limits on the retention of the data associated with the instances (e.g., were individuals in question told that their data would be retained for a fixed period of time and then deleted)?}{If so, please describe these limits and explain how they will be enforced.}
\label{Q56}

\dsanswer{Objaverse and ABO. N/A}
    %Some images in \dsetname{} may depict people (\qref{Q17}).
    %Rather then directly distributing images, we distribute URLs that point to the original images uploaded by Reddit users.
    %This means that users retain full control of their data -- any post deleted from Reddit will be automatically removed from \dsetname{} (see also \qref{Q10}, \qref{Q14}, \qref{Q31}).
}

\dsquestionex{Will older versions of the dataset continue to be supported/hosted/maintained?}{If so, please describe how. If not, please describe how its obsolescence will be communicated to users.}
\label{Q57}

\dsanswer{Objaverse and ABO. Old versions will continue to be available on the Hugging Face; its obsolescence will be announced along with the new version on the project website. The exception will be if the dataset is updated per ethical concerns or upon user request (see \ref{Q55}), in which case the older version will be depricated for ethical reasons.
}

\dsquestionex{If others want to extend/augment/build on/contribute to the dataset, is there a mechanism for them to do so?}{If so, please provide a description. Will these contributions be verified? If so, please describe how. If not, why not? Is there a process for communicating/distributing these contributions to other users? If so, please provide a description.}
\label{Q58}

\dsanswer{Objaverse and ABO. Yes, others can build upon this dataset. We share our captioning code as well as instructions for human annotation. These processes could be used to not only obtain additional captions for the same data, but can be used to collect future datasets as 3D assets become available at larger scale. These contributions could be verified automatically through some of the methods used in the paper e.g. CLIPScore~\cite{hessel2021clipscore,radford2021learning}. The contributions can also easily be shared via a dict mapping ID to caption.
}

\end{compactenum}
