# Supplementary material for: Scalable 3D Captioning with Pretrained Models
Source: arXiv:2306.07279 source file (2023-06-16)
Supplement: Supplementary file 3 [file caption_abo.tex]

\begin{table}
\caption{\textbf{Automated Captioning Metrics on ABO}. Automated metrics .}
\label{tab:caption_abo}
\resizebox{\ifdim\width>\linewidth \linewidth \else \width \fi}{!}{
\begin{tabular}{lccccccccc}
\toprule
% & \multicolumn{4}{c}{Objaverse} \\
%\multirow{2}{*}{Method} & \multicolumn{3}{c}{A/B} & CLIP & ViLBERT & \multirow{2}{*}{TIGER} \\ 
\multirow{2}{*}{Method} & A/B & A/B & A/B & CLIP & \multicolumn{2}{c}{ViLT Image Retr.} & \multicolumn{2}{c}{ViLT Text Retr.} \\ 
 & Score (1-5) & Win vs. Ours & Lose vs. Ours & Score & R@5 & R@10 & R@5 & R@10 \\
\midrule
BLIP2 & 2.87 \pm 0.019 & 41.0\% \pm 0.7\% & 50.6\% \pm 0.7\% & 83.1 & 24.7 & 32.3 & 21.9 & 29.3 \\
+ GPT4 & 2.99 \pm 0.018 & 37.3\% \pm 0.7\% & 39.3\% \pm 0.7\% & 86.3 & \textbf{31.9} & 39.9 & 30.2 & 38.4 \\
+ CLIP (Ours) & \textbf{-} & \textbf{-} & \textbf{-} & \textbf{86.9} & 31.1 & \textbf{40.2} & \textbf{30.3} & \textbf{38.6} \\
\bottomrule
\end{tabular}
}
\end{table}
