# Supplementary material for: Scalable 3D Captioning with Pretrained Models
Source: arXiv:2306.07279 source file (2023-06-16)
Supplement: Supplementary file 4 [file objaverse_analysis.tex]

\begin{table}[t]
\captionsetup{type=figure}
\centering
\begin{minipage}{.5\textwidth}
  \centering
  %\captionsetup{width=0.95\textwidth}
  %\caption{\textbf{Objaverse Human Caption Comparison}. N-grams are per 1k captions. Our captions contain a smaller vocabulary and longer length than human captions.}
    \resizebox{\ifdim\width>\linewidth \linewidth \else \width \fi}{!}
    {
    \begin{tabular}{lccc}
        \toprule
        & \multicolumn{3}{c}{\textit{Occurrences in 39k captions}} \\
        \textbf{Captions} & \textbf{Unigrams} & \textbf{Bigrams} & \textbf{Trigrams} \\
        \midrule
        % divide by 38714
        Metadata & 58,490 & 237,958 & 377,425 \\
        Human & 10,659 & 80,552 & 161,583 \\
        Ours & 8,438 & 54,176 & 129,810 \\
        %Metadata & 1,511 & 6,146 & 9,749 \\
        %Human & 275 & 2,081 & 4,174 \\
        %Ours & 218 & 1,399 & 3,353 \\
        %Metadata & 151 & 615 & 975 \\
        %Human & 28 & 208 & 417 \\
        %Ours & 22 & 140 & 335 \\
        \bottomrule
    \end{tabular}
    }
    {
    \includegraphics[width=\linewidth]{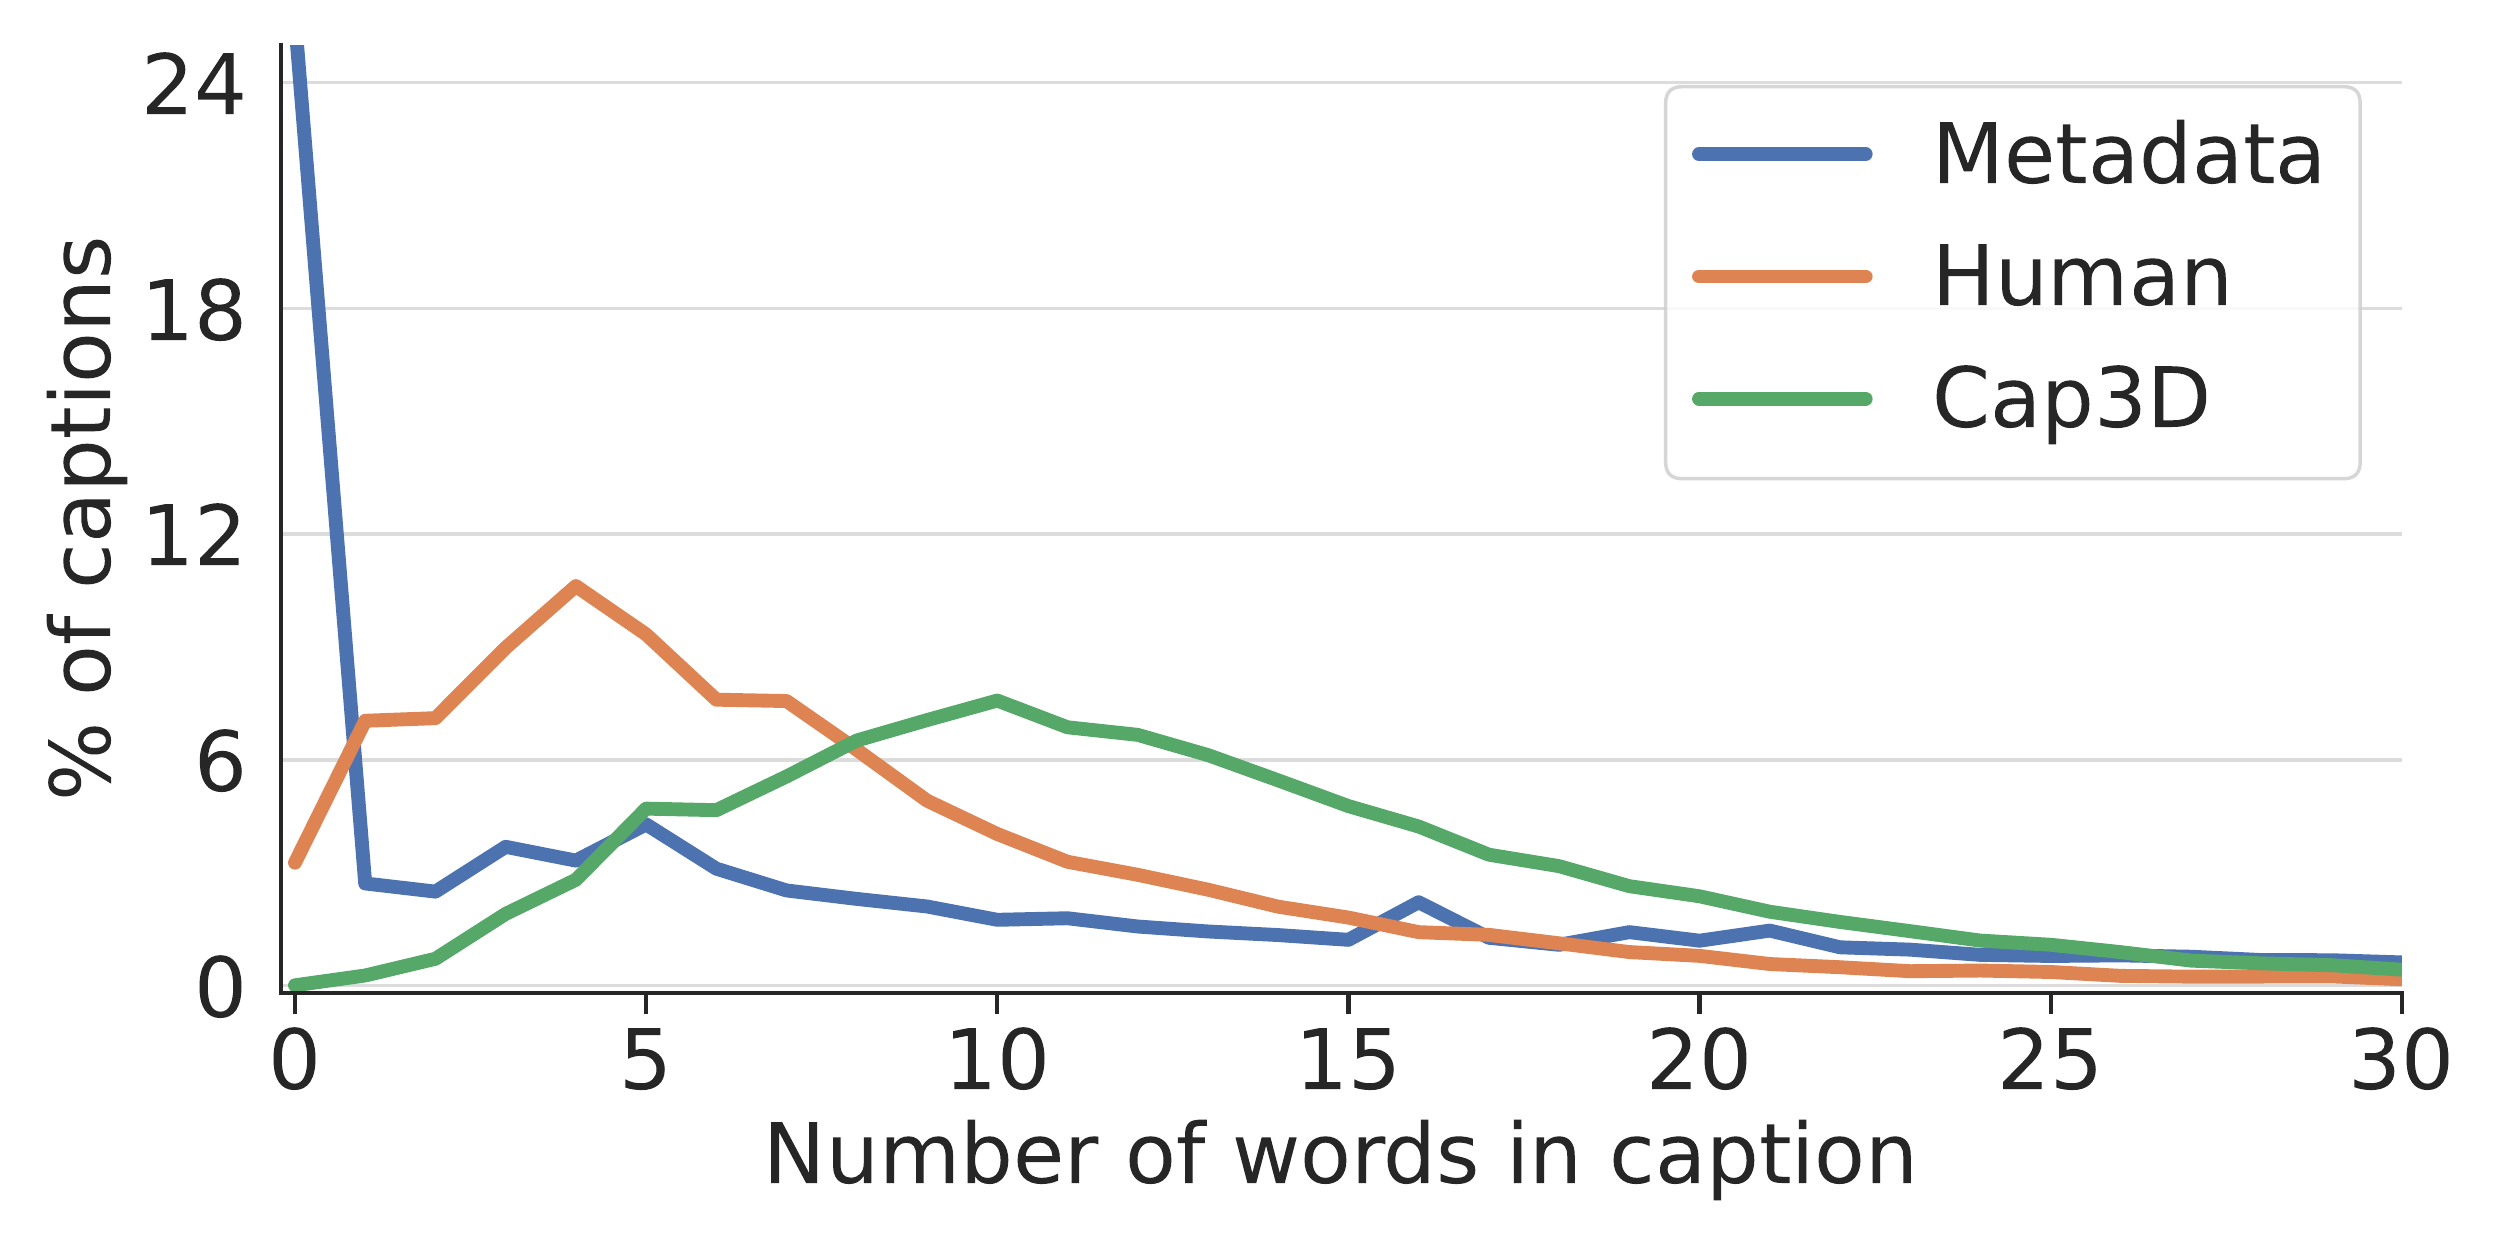}
    }
    \captionsetup{width=0.95\textwidth}
  \caption{\textbf{Objaverse Human Caption}. Our captions contain a smaller vocabulary and longer length than human captions. Metadata has a long tail of vocabulary and length.}
  \label{fig:objaverse_analysis_human}
\end{minipage}%
\begin{minipage}{.5\textwidth}
  \centering
  %\captionsetup{width=0.95\textwidth}
  %\caption{\textbf{Objaverse Automated Caption Comparison}. N-grams are per 1k captions. GPT produces longer and more varied captions than BLIP2; CLIP tends to prune incorrect details and reduces length slightly.}
      
    \resizebox{\ifdim\width>\linewidth \linewidth \else \width \fi}{!}
    {
    \begin{tabular}{lccc}
        \toprule
        & \multicolumn{3}{c}{\textit{Occurrences in 5k captions}} \\
        \textbf{Captions} & \textbf{Unigrams} & \textbf{Bigrams} & \textbf{Trigrams} \\
        \midrule
        % divide by 5000
        BLIP2 & 1,619 & 6,043 & 9,986 \\
        + GPT 4 & 3,409 & 16,187 & 32,127 \\
        + CLIP (Cap3D) & 3,292 & 14,800 & 28,200 \\
        %BLIP2 & 324 & 1,209 & 1,997 \\
        %+ GPT 4 & 682 & 3,237 & 6,425 \\
        %+ CLIP (Ours) & 658 & 2,960 & 5,640 \\
        %BLIP2 & 32 & 121 & 200 \\
        %+GPT 4 & 68 & 324 & 643 \\
        %+CLIP(Ours) & 66 & 296 & 564 \\
        \bottomrule
    \end{tabular}
    }
    {
    \includegraphics[width=\linewidth]{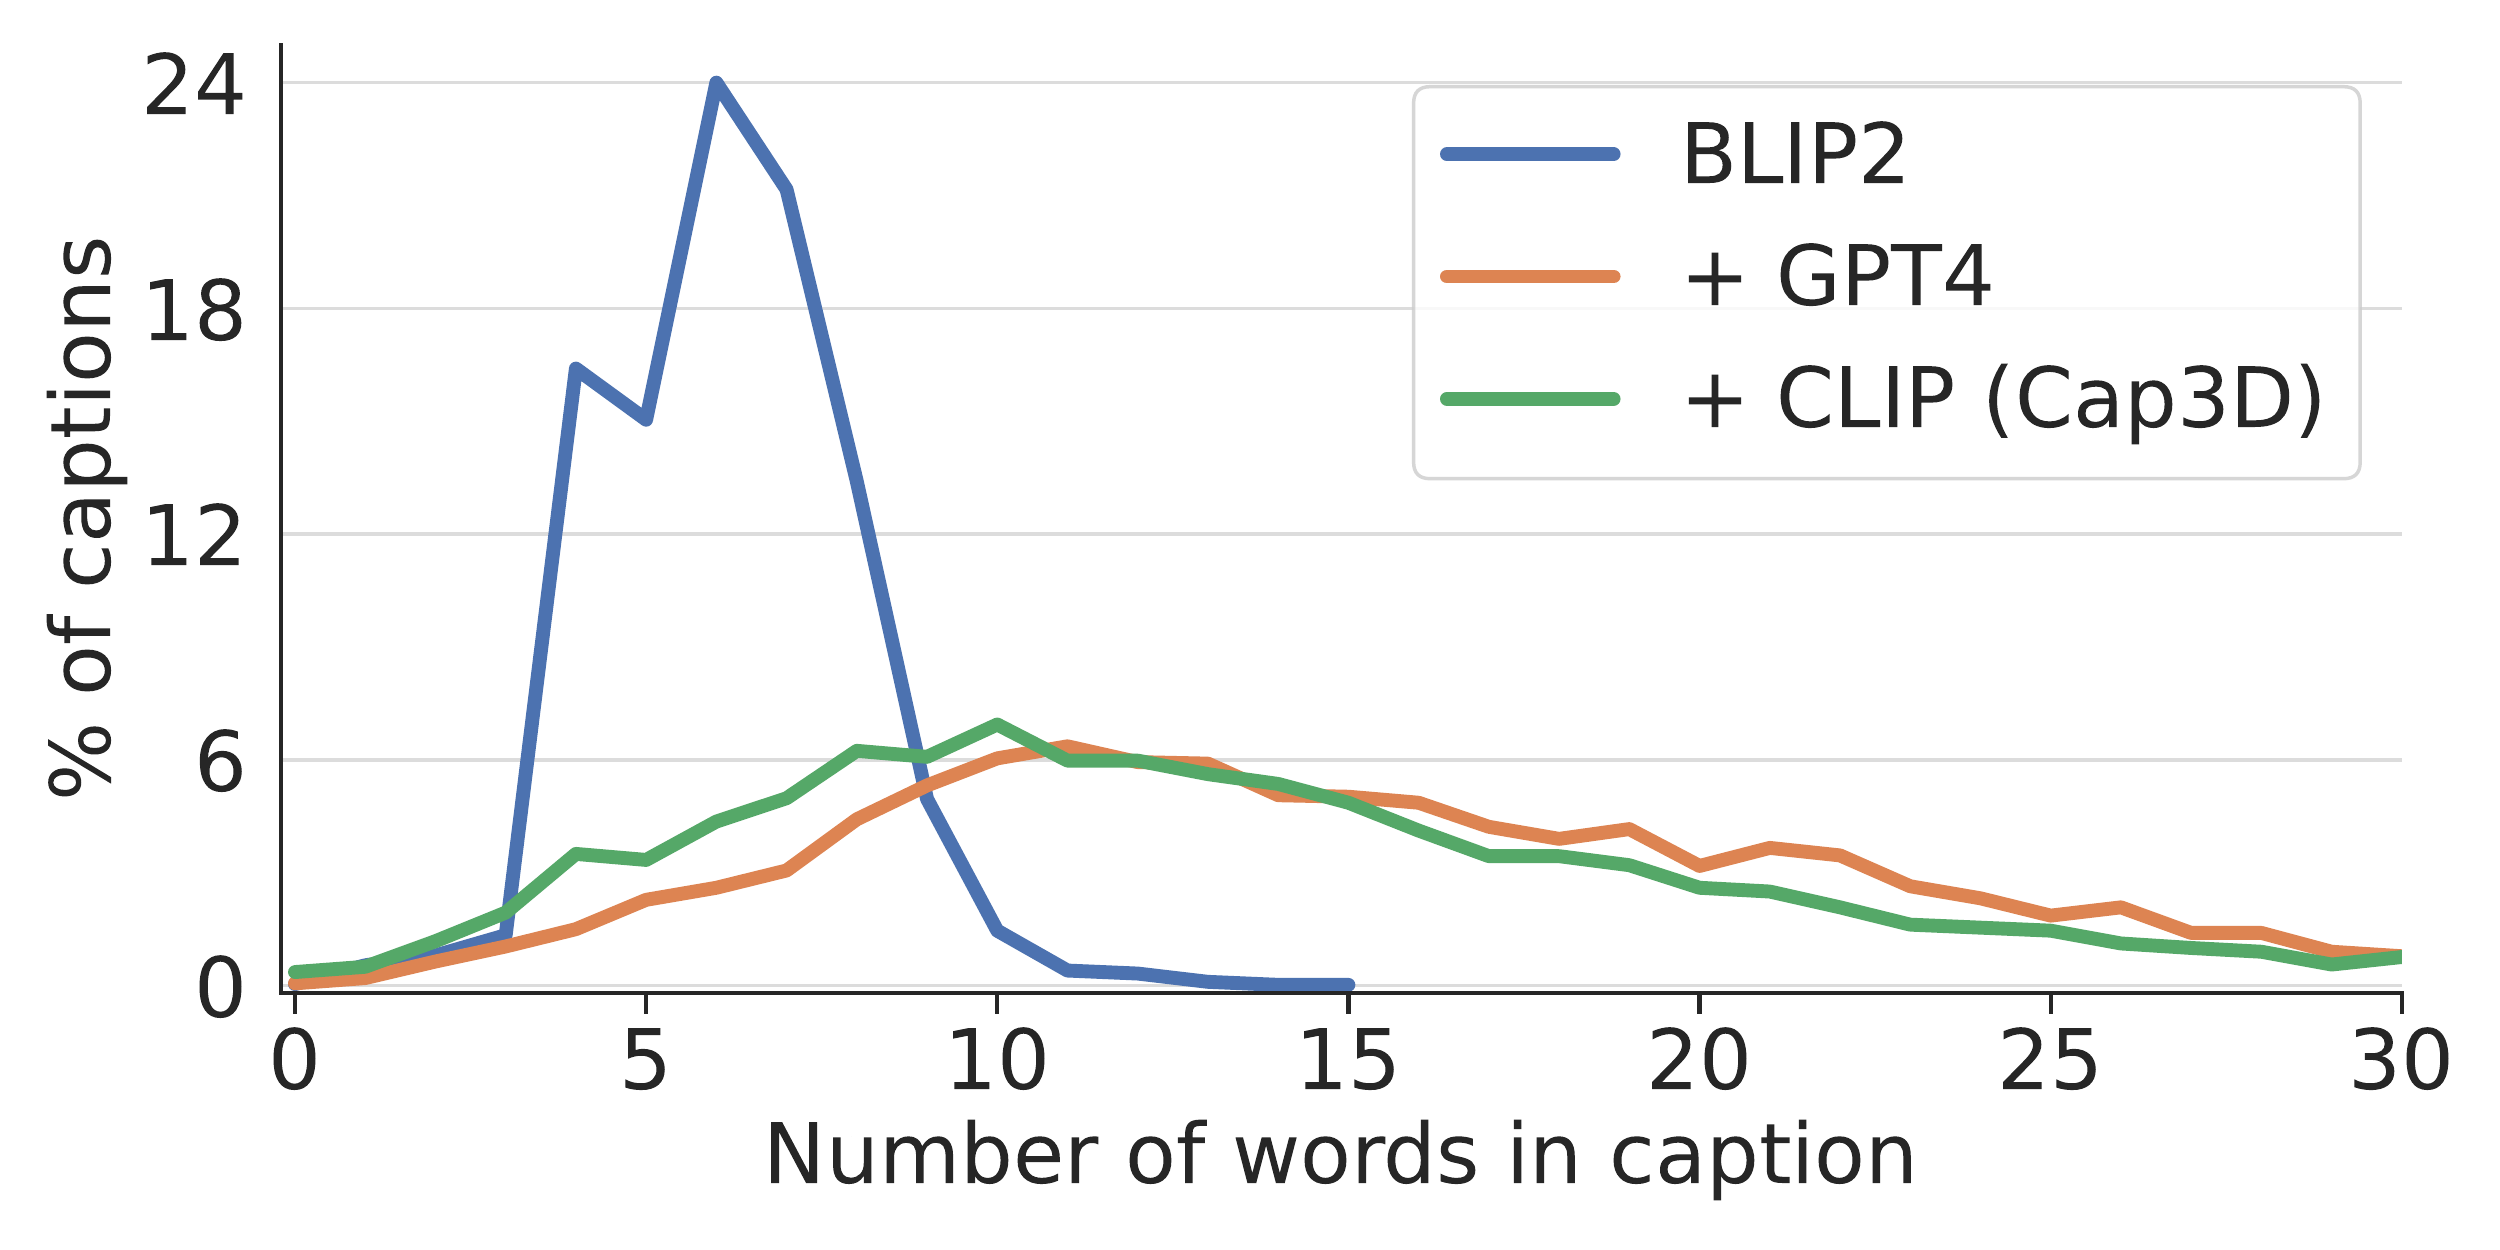}
    \captionsetup{width=0.95\textwidth}
    \caption{\textbf{Objaverse Automated Caption}. GPT produces longer and more varied captions than BLIP2; CLIP tends to prune incorrect details and reduces length slightly.}
  }
  \label{fig:objaverse_analysis_automated}
\end{minipage}
\end{table}
